# Supplementary material for: The Blessings of Multiple Treatments and Outcomes in Treatment Effect Estimation
Source: arXiv:2309.17283 source file (2023-10-14)
Supplement: Supplementary file 1 [file appE.tex]

\section{Hypothesis Testing Experiments}
In this appendix, we report the results of hypothesis testing Experiments. 
\subsection{Confounding strength}
Unknown confounding strength affects the results of our method differently in different cases. We considre the toy examples intuitively

\noindent\textbf{Data generation.} We describe the data generating mechanism of toy example. First, $U\sim N(0,1)$, We consider the example and consider the details of the

% : 1) independent case: when two variables are independent; 2) causal relationship: when there is a causal relationship between two variables.

% To understand the results, we could analyze some toy examples intuitively. The first experiment should satisfy the structural equations as follows:
\begin{itemize}[topsep=0.1pt,leftmargin=0.4cm]
    \item $U$: $U\sim N(0,1)$
    \item $A$: $A = \beta \times U + \varepsilon_1$ where $\varepsilon_1 \sim N(0,1)$ 
    \item $W$: $W = \beta \times U +\varepsilon_2$ where $\varepsilon_3 \sim N(0,1)$ 
    \item causal case: $Y = A+W+\beta \times U + \varepsilon_3$ where $\varepsilon_3 \sim N(0,1)$. independent case: $Y = W+\beta \times U + \varepsilon_3$ where $\varepsilon_3 \sim N(0,1)$ .  
\end{itemize}

The second experiment should satisfy the structural equations as follows
\begin{itemize}[topsep=0.1pt,leftmargin=0.4cm]
    \item $U$: $U\sim N(0,1)$
    \item $A$: $A = \beta \times U + \varepsilon_1$ where $\varepsilon_1 \sim N(0,1)$ 
    \item $W$: $W = \beta \times U +\varepsilon_2$ where $\varepsilon_3 \sim N(0,1)$ 
    \item causal case: $Y = A+W +\beta \times \tanh(U) + \varepsilon_3$ where $\varepsilon_3 \sim N(0,1)$. independent case: $Y = W+\beta \times \tanh(U) + \varepsilon_3$ where $\varepsilon_3 \sim N(0,1)$ .  
\end{itemize}

We generat a dataset comprising 1000 samples for each FCM. To ensure a comprehensive analysis, we divide $W$ into 10 bins and $A$ into 14 bins, respectively. We then compute the corresponding $p$-values. In order to evaluate type I and type II errors more effectively and reduce randomness, we repeate the experiment 50 times. 

To explore the impact of Confounding variable strength, we vary the coefficient of the Confounding variables, denoted as $\beta$, across different values: 0.1, 1, 10, 20, and 100. By altering the strength of the confounding variables, we aim to assess their influence on the hypothesis testing.

\begin{table}[htbp]
  \centering
  \caption{The experimental results of the first experiment in the presence of confounding variables of different strengths.}
    \begin{tabular}{c|cc|cc}
    \hline
    \multirow{2}{*}{Confounding strength} & \multicolumn{2}{c|}{Causal} & \multicolumn{2}{c}{Independent} \\
\cline{2-5}          & \multicolumn{1}{c|}{$p$-value} & Type I error & \multicolumn{1}{c|}{$p$-value} & Type II error \\
    \hline
    $\beta=0.1$  & 0.006  & 0.040  & 0.607  & 0.030  \\
    $\beta=1$ & 0.002  & 0.010  & 0.525  & 0.060  \\
    $\beta=10$ & 0.044  & 0.120  & 0.147  & 0.520  \\
    $\beta=20$ & 0.067  & 0.330  & 0.123  & 0.450  \\
    $\beta=100$ & 0.092  & 0.280  & 0.109  & 0.360  \\
    \hline
    \end{tabular}%
  \label{tab:exp1}%
\end{table}%

\begin{table}[htbp]
  \centering
  \caption{The experimental results of the second experiment in the presence of confounding variables of different strengths.}
    \begin{tabular}{c|cc|cc}
    \hline
    \multirow{2}{*}{Confounding strength} & \multicolumn{2}{c|}{Causal} & \multicolumn{2}{c}{Independent} \\
\cline{2-5}          & \multicolumn{1}{c|}{$p$-value} & Type I error & \multicolumn{1}{c|}{$p$-value} & Type II error \\
    \hline
    $\beta=0.1$ & 0.006  & 0.040  & 0.607  & 0.050  \\
    $\beta=1$ & 0.004  & 0.010  & 0.564  & 0.060  \\
    $\beta=10$ & 0.030  & 0.100  & 0.156  & 0.450  \\
    $\beta=20$& 0.063  & 0.190  & 0.136  & 0.570  \\
    $\beta=100$ & 0.089  & 0.250  & 0.112  & 0.640  \\
    \hline
    \end{tabular}%
  \label{tab:exp2}%
\end{table}%

Regarding the experimental results, we find that confounding variable strength affects both independent and causal cases. When $\beta$ is small, the strength of the confounding variable becomes smaller than that of the proxy variable. As a result, the confounding variable $U$ can be effectively explained by the proxy variable, enabling hypothesis testing to be conducted effectively. However, as $\beta$ increases, the influence of the confounding variable becomes dominant and cannot be adequately explained through the proxy variables. This, in turn, affects the accuracy of our experimental results and leads to an increase in both the first and second types of errors. Moreover, we observe that the nonlinear function will make the growth trend of the first and second types of errors larger.

\subsection{Proxy strength}
We highlight the potential consequences of exceptionally weak strength in the proxy variable, as it could potentially lead to incorrect conclusions in hypothesis testing. To further investigate this issue, we conduct a series of toy experiments aimed at exploring the impact of proxy variable strength on the process of hypothesis testing.

The first experiment should satisfy the structural equations as follows:
\begin{itemize}[topsep=0.1pt,leftmargin=0.4cm]
    \item $U$: $U\sim N(0,1)$
    \item $A$: $A = U + \varepsilon_1$ where $\varepsilon_1 \sim N(0,1)$ 
    \item $W$: $W =\beta\times U +\varepsilon_2$ where $\varepsilon_2 \sim N(0,1)$ 
    \item causal case: $Y = A + U + \varepsilon_3$ where $\varepsilon_3 \sim N(0,1)$. independent case: $Y = U + \varepsilon_3$ where $\varepsilon_3 \sim N(0,1)$ .  
\end{itemize}
The second experiment should satisfy the structural equations as follows
\begin{itemize}[topsep=0.1pt,leftmargin=0.4cm]
    \item $U$: $U\sim N(0,1)$
    \item $A$: $A = U + \varepsilon_1$ where $\varepsilon_1 \sim N(0,1)$ 
    \item $W$: $W =\beta\times \tanh{U} +\varepsilon_2$ where $\varepsilon_2 \sim N(0,1)$ 
    \item causal case: $Y = A + U + \varepsilon_3$ where $\varepsilon_3 \sim N(0,1)$. independent case: $Y = U + \varepsilon_3$ where $\varepsilon_3 \sim N(0,1)$ .  
\end{itemize}

We generate a dataset comprising 1000 samples for each FCM. To ensure a comprehensive analysis, we divide $W$ into 10 bins and $A$ into 14 bins, respectively. We then compute the corresponding $p$-values. In order to evaluate type I and type II errors more effectively and reduce randomness, we repeate the experiment 50 times. 

To explore the impact of proxy variable strength, we variy the coefficient of the proxy variables, denoted as $\beta$, across different values: 0.1, 1, 10, 20, and 100. By altering the strength of the proxy variables, we aim to assess their influence on the hypothesis testing.

\begin{table}[htbp]
  \centering
  \caption{The experimental results of the first experiment in the presence of proxy variables of different strengths.}
    \begin{tabular}{c|cc|cc}
    \hline
    \multirow{2}{*}{Proxy strength} & \multicolumn{2}{c|}{Causal} & \multicolumn{2}{c}{Independent} \\
\cline{2-5}          & \multicolumn{1}{c|}{$p$-value} & \multicolumn{1}{c|}{Type II error} & \multicolumn{1}{c|}{$p$-value} & \multicolumn{1}{c}{Type I error} \\
    \hline
    $\beta=0.1$ & 5.24E-19 & 0.000     & 0.019  & 0.910 \\
    $\beta=1$ & 1.65E-06 & 0.000     & 0.370  & 0.150 \\
    $\beta=10$ & 0.018  & 0.060  & 0.561  & 0.010 \\
   $\beta=20$ & 0.024 & 0.070  & 0.556  & 0.030 \\
    $\beta=100$ & 0.022 & 0.070   & 0.560  & 0.050 \\
    \hline
    \end{tabular}%
  \label{experiment-proxy_linear}%
\end{table}%

\begin{table}[htbp]
  \centering
  \caption{The experimental results of the second experiment in the presence of proxy variables of different strengths.}
    \begin{tabular}{c|cc|cc}
    \hline
    \multirow{2}{*}{Proxy strength} & \multicolumn{2}{c|}{Causal} & \multicolumn{2}{c}{Independent} \\
\cline{2-5}          & \multicolumn{1}{c|}{$p$-value} & \multicolumn{1}{c|}{Type II error} & \multicolumn{1}{c|}{$p$-value} & \multicolumn{1}{c}{Type I error} \\
    \hline
    $\beta=0.1$ & 1.12E-16 & 0.000     & 0.008 & 0.950 \\
    $\beta=1$ & 5.92E-06 & 0.000     & 0.159 & 0.460 \\
    $\beta=10$ & 0.01256 & 0.070  & 0.546 & 0.050 \\
    $\beta=20$ & 0.017 & 0.070  & 0.526 & 0.060 \\
    $\beta=100$ & 0.022 & 0.090  & 0.513 & 0.040 \\
    \hline
    \end{tabular}%
  \label{experiment-proxy_nonlinear}%
\end{table}%

Regarding the experimental results, we find that in the independent case, the strength of the proxy variable has a more pronounced impact on the outcomes, which differs from the causal case. In the independent case, as the proxy strength diminishes, its ability to explain the variable $U$ decreases. Consequently, it becomes challenging to utilize the proxy variable as a means to assess independence. However, in the causal scenario, the relationship between variable $A$ and variable $Y$ is related with a confounding variable $U$. Moreover,
we find that non-linear functions can make it more difficult to infer independent relationships, thus requiring strong proxy variables.

\subsection{Robustness to different distribution}

We use different hypothesized noise distributions to test the robustness to the misspecification of noise distribution.

\begin{itemize}[topsep=0.1pt,leftmargin=0.4cm]
    \item $U$: $\varepsilon_1$
    \item $A$: $A = U + \varepsilon_2$ 
    \item $W$: $W =\beta\times U +\varepsilon_3$ 
    \item causal case: $Y = A + U + \varepsilon_4$. independent case: $Y = U + \varepsilon_4$.  
\end{itemize}
where $\varepsilon_i(i=1,2,3,4)$ is one of the four hypothesized distributions: uniform distribution $U(0, 1)$, beta distribution $\mathcal{B}(a=4,b=4)$, exponential distribution $E(\lambda=1)$ and standard normal distribution $N(0, 1)$.

We generate a dataset comprising 1000 samples for each FCM. To ensure a comprehensive analysis, we divide $W$ into 10 bins and $A$ into 14 bins, respectively. We then compute the corresponding $p$-values. In order to evaluate type I and type II errors more effectively and reduce randomness, we repeate the experiment 50 times.

\begin{table}[htbp]
  \centering
  \caption{The experimental results in the presence of different noise.}
    \begin{tabular}{c|cc|cc}
    \hline
    \multirow{2}{*}{Hypothesized distributions} & \multicolumn{2}{c|}{Causal} & \multicolumn{2}{c}{Independent} \\
\cline{2-5}          & \multicolumn{1}{c|}{$p$-value} & \multicolumn{1}{c|}{Type II error} & \multicolumn{1}{c|}{$p$-value} & \multicolumn{1}{c}{Type I error} \\
    \hline
    Uniform & 1.14E-10 & 0.000  & 0.512  & 0.070  \\
    Beta  & 5.05E-06 & 0.000  & 0.408  & 0.140  \\
    Exponential & 8.00E-04  & 0.010  & 0.321  & 0.280  \\
    Norm  & 1.65E-06  & 0.000  & 0.370  & 0.150  \\
    \hline
    \end{tabular}%
  \label{experiment-noise}%
\end{table}%

Regarding the experimental results, we find that in the independent case, different noise has a more pronounced impact on the outcomes, which differs from the causal case. In the independent case, our findings indicate that the first and second types of errors associated with the uniform distribution are minimal. This observation can be attributed to the fact that the uniform distribution is a bounded random variable. However, for other unbounded distributions, truncating the processing introduces certain deviations that lead to an increase in the first type of error. In the causal scenario, the relationship between variable $A$ and variable $Y$ is related with a confounding variable $U$.
